# Supplementary material for: Beyond Complete Shapes: A Benchmark for Quantitative Evaluation of 3D Shape Surface Matching Algorithms
Source: arXiv:2411.03511 source file (2025-11-24)
Supplement: Supplementary file 1 [file tab_datasets_licenses.tex]

\begin{table}[tbh!]
\centering
\footnotesize
\begin{tabular}{lcc}
\toprule
\textbf{Dataset}  & \textbf{License} & \textbf{Website}  \\
\midrule
FAUST~\cite{bogo2014faust}          & {\color[HTML]{0065bd} \href{https://faust-leaderboard.is.tuebingen.mpg.de/license}{License link}}  &   {\color[HTML]{0065bd} \href{https://faust-leaderboard.is.tuebingen.mpg.de/}{Project page}}     \\
SCAPE~\cite{anguelov2005scape}      & N.A.   &   {\color[HTML]{0065bd} \href{https://ai.stanford.edu/~drago/Projects/scape/scape.html}{Project page}}     \\
KIDS~\cite{rodola2014dense}         &  N.A.  &   {\color[HTML]{0065bd} \href{https://cvg.cit.tum.de/data/datasets/kids}{Project page}}     \\
SMAL~\cite{Zuffi:CVPR:2017}         & {\color[HTML]{0065bd} \href{https://smal.is.tue.mpg.de/license.html}{License link}}  &   {\color[HTML]{0065bd} \href{https://smal.is.tue.mpg.de/index.html}{Project page}}     \\
SHREC'20~\cite{dyke2020shrec}       & N.A. &   {\color[HTML]{0065bd} \href{http://robertodyke.com/shrec2020/index2.html}{Project page}}     \\
DT4D~\cite{li20214dcomplete}        & {\color[HTML]{0065bd} \href{https://docs.google.com/forms/d/e/1FAIpQLSckMLPBO8HB8gJsIXFQHtYVQaTPTdd-rZQzyr9LIIkHA515Sg/viewform}{License link}}  &   {\color[HTML]{0065bd} \href{https://github.com/rabbityl/DeformingThings4D}{Project page}}     \\
TOSCA~\cite{bronstein2008numerical} & N.A.    & We have permission    \\
                                                      &                          &  to distribute \\
\bottomrule
\end{tabular}
\caption{\textbf{List of licenses of all datasets} used in the \bm{} benchmark. SCAPE, KIDS, SHREC'20 and TOSCA do not have explicit licenses. We got permission from the original authors of TOSCA to distribute the assets on our GitHub repository.}
\label{tab:dataset_licenses}
\end{table}
